# Supplementary material for: Commonsense Video Question Answering through Video-Grounded Entailment Tree Reasoning
Source: arXiv:2501.05069 source file (2025-03-25)
Supplement: Supplementary file 1 [file supp_breakdown_gnd.tex]

% Please add the following required packages to your document preamble:
% \usepackage{graphicx}
\begin{table}[t]
\centering
\resizebox{0.6\linewidth}{!}{%
\begin{tabular}{cc|cc}
\hline
\multicolumn{2}{c|}{Components}              & \multicolumn{2}{c}{Acc} \\ \hline
\begin{tabular}[c]{@{}c@{}}Fact-condition \\ captioning\end{tabular} & \begin{tabular}[c]{@{}c@{}}Structure-based \\ retrieval\end{tabular} & Original & Rewritten \\ \hline
\multicolumn{1}{l}{} & \multicolumn{1}{l|}{} & 56.2       & 49.6       \\
$\checkmark$                  &                       & 59.5       & 53.3       \\
                     & $\checkmark$                   & 58.4       & 52.7       \\
$\checkmark$                  & $\checkmark$                   & 60.5       & 55.4       \\ \hline
\end{tabular}%
}
\caption{Ablation study of our grounding part.}
\label{tab:supp_break_ground}
\end{table}
