# Supplementary material for: Commonsense Video Question Answering through Video-Grounded Entailment Tree Reasoning
Source: arXiv:2501.05069 source file (2025-03-25)
Supplement: Supplementary file 2 [file supp_combination.tex]

\begin{table}[t!]
\centering
\vspace{-3pt}
\begin{minipage}[t]{\linewidth}
\centering
\resizebox{\linewidth}{!}{%
\begin{tabular}{c|cc|cccc}
\hline
\multirow{2}{*}{Method} & \multicolumn{2}{c|}{General VLM} & \multicolumn{4}{c}{VQA approaches}             \\ \cline{2-7} 
                        & VideoChat2      & VideoLlaVA     & VideoAgent & VideoTree & LLoVi & Ours          \\ \hline
Inf time(s)                & 7.5             & 6.2            & 51.0       & 34.6      & 40.3  & 38.2          \\ \hline
Avg acc                 & 49.0            & 50.8           & 61.6       & 60.9      & 58.6  & \textbf{62.6} \\ \hline
Reasoner &
  \begin{tabular}[c]{@{}c@{}}VideoChat2\\ (7B)\end{tabular} &
  \begin{tabular}[c]{@{}c@{}}VideoLlaVA\\ (7B)\end{tabular} &
  \begin{tabular}[c]{@{}c@{}}GPT-4\\ (1.8T)\end{tabular} &
  \begin{tabular}[c]{@{}c@{}}GPT-4\\ (1.8T)\end{tabular} &
  \begin{tabular}[c]{@{}c@{}}GPT-4\\ (1.8T)\end{tabular} &
  \begin{tabular}[c]{@{}c@{}}VideoLlaVA\\ (\textbf{7B})\end{tabular} \\ \hline
\end{tabular}%
}
\vspace{-10pt}
\caption{Efficiency comparison. The average inference time for each video is reported.}
\label{tab:supp_efficiency}
\end{minipage}
\begin{minipage}[t]{0.5\linewidth}
\resizebox{\linewidth}{!}{%
\begin{tabular}{cc|cc}
\hline
\multicolumn{2}{c|}{Components}              & \multicolumn{2}{c}{Acc} \\ \hline
\begin{tabular}[c]{@{}c@{}}Fact-\\ conditioned \\ captioning\end{tabular} & \begin{tabular}[c]{@{}c@{}}Structure-\\ based \\ retrieval\end{tabular} & Original & Rewritten \\ \hline
\multicolumn{1}{l}{} & \multicolumn{1}{l|}{} & 56.2       & 49.6       \\
yes                  &                       & 59.5       & 53.3       \\
                     & yes                   & 58.4       & 52.7       \\
yes                  & yes                   & 60.5       & 55.4       \\ \hline
\end{tabular}%
}
\vspace{-10pt}
\caption{Ablation study of main components in grounding part.}
\label{tab:supp_break_ground}
\end{minipage}
\hfill
\begin{minipage}[t]{0.48\linewidth}
    \centering
    \begin{minipage}[t]{\linewidth}
    \centering
    \vspace{-1.3cm}
    \resizebox{\textwidth}{!}{%
    \begin{tabular}{c|c|c}
    \hline
    Method          & Original set & De-basing set \\ \hline
    Human w/o video & 79.3         & 44.6          \\ \hline
    Human w/ video  & 96.4         & 93.9          \\ \hline
    \end{tabular}}
    \vspace{-10pt}
        \caption{Results of subjective human evaluation (NExT-QA).}
        \label{tab:supp_quality}
    \end{minipage}
    \vspace{1cm}
    \begin{minipage}[t]{\linewidth}
    \centering
    \resizebox{0.9\textwidth}{!}{%
    \begin{tabular}{c|c|c|c}
    \hline
    Model       & NExT-QA & IntentQA & Avg                          \\ \hline
    VideoLlaMA3 & 61.4    & 59.7     & 60.6                         \\
    \rowcolor[HTML]{E2E1E1} 
    +Ours       & 63.2    & 60.9     & \cellcolor[HTML]{E2E1E1}62.1 \\ \hline
    \end{tabular}%
    }
    \vspace{-10pt}
        \caption{Results of VideoLlaMA3 w/ Ours.}
        \label{tab:supp_videollama3}
    \end{minipage}
    \end{minipage}
    \vspace{-1.3cm}
\end{table}
