# Supplementary material for: Commonsense Video Question Answering through Video-Grounded Entailment Tree Reasoning
Source: arXiv:2501.05069 source file (2025-03-25)
Supplement: Supplementary file 3 [file supp_human.tex]

% Please add the following required packages to your document preamble:
% \usepackage{graphicx}
\begin{table}[t]
\centering
\resizebox{0.6\linewidth}{!}{%
\begin{tabular}{c|c|c}
\hline
Method          & Original set & De-basing set \\ \hline
Human w/o video & 79.3         & 44.6          \\ \hline
Human w/ video  & 96.4         & 93.9          \\ \hline
\end{tabular}%
}
\caption{Average results of the original set and de-basing set, which are answered by 3 people under (1) only observing the question-answers (2) watching both the video and question-answers}
\label{tab:supp_quality}
\end{table}
