# Supplementary material for: Commonsense Video Question Answering through Video-Grounded Entailment Tree Reasoning
Source: arXiv:2501.05069 source file (2025-03-25)
Supplement: Supplementary file 4 [file supp_time.tex]

% Please add the following required packages to your document preamble:
% \usepackage{multirow}
% \usepackage{graphicx}
\begin{table}[t]
\centering
\resizebox{\linewidth}{!}{%
\begin{tabular}{c|cc|cccc}
\hline
\multirow{2}{*}{Method} & \multicolumn{2}{c|}{General VLM} & \multicolumn{4}{c}{VQA approaches}             \\ \cline{2-7} 
                        & VideoChat2      & VideoLlaVA     & VideoAgent & VideoTree & LLoVi & Ours          \\ \hline
Inf time(s)                & 7.5             & 6.2            & 51.0       & 34.6      & 40.3  & 38.2          \\ \hline
Avg acc                 & 49.0            & 50.8           & 61.6       & 60.9      & 58.6  & \textbf{62.6} \\ \hline
Reasoner &
  \begin{tabular}[c]{@{}c@{}}VideoChat2\\ (7B)\end{tabular} &
  \begin{tabular}[c]{@{}c@{}}VideoLlaVA\\ (7B)\end{tabular} &
  \begin{tabular}[c]{@{}c@{}}GPT-4\\ (1.8T)\end{tabular} &
  \begin{tabular}[c]{@{}c@{}}GPT-4\\ (1.8T)\end{tabular} &
  \begin{tabular}[c]{@{}c@{}}GPT-4\\ (1.8T)\end{tabular} &
  \begin{tabular}[c]{@{}c@{}}VideoLlaVA\\ (\textbf{7B})\end{tabular} \\ \hline
\end{tabular}%
}
\caption{Efficiency comparison. The average inference time for each video is reported. Acc is reported by the average accuracy on the de-biasing set of NExT-QA and Intent-QA.}
\label{tab:supp_efficiency}
\end{table}

%Efficiency comparison. The average inference time for each video in NExT-QA is reported.
