# Supplementary material for: Commonsense Video Question Answering through Video-Grounded Entailment Tree Reasoning
Source: arXiv:2501.05069 source file (2025-03-25)
Supplement: Supplementary file 5 [file supp_videollama3.tex]

% Please add the following required packages to your document preamble:
% \usepackage{graphicx}
% \usepackage[table,xcdraw]{xcolor}
% Beamer presentation requires \usepackage{colortbl} instead of \usepackage[table,xcdraw]{xcolor}
\begin{table}[t]
\centering
\resizebox{0.6\linewidth}{!}{%
\begin{tabular}{c|c|c|c}
\hline
Model       & NExT-QA & IntentQA & Avg                          \\ \hline
VideoLlaMA3 & 61.4    & 59.7     & 60.6                         \\
\rowcolor[HTML]{E2E1E1} 
+Ours       & 63.2    & 60.9     & \cellcolor[HTML]{E2E1E1}62.1 \\ \hline
\end{tabular}%
}
\caption{Results of VideoLlaMA3 incorporating our framework.}
\label{tab:supp_videollama3}
\end{table}
